# Supplementary material for: CommerceMM: Large-Scale Commerce MultiModal Representation Learning with Omni Retrieval
Source: arXiv:2202.07247 source file (2022-02-15)
Supplement: Supplementary file 1 [file 5.appendix.tex]

\section{Appendix}
\subsection{Training Details}
During pre-training, we set the learning rate as 5e-5, batch size as 2,048, and update in total 300K steps.
We apply another 100K steps for a 2nd-stage pre-training when modality randomization is applied.
In the 5 image-text pre-training tasks, we assign equal weights to MIM-kl, MIM-fr, ITM and ITC and half of their weights to MLM.
We found equal weight on MLM will hurt the overall performance.
One possible reason is MLM's effectivenss is overshadowed by the more effective MIM tasks.
For the 9 Omni-Retrieval tasks, we also assign the same weight to each of them.
Our model is trained in a round-robin fashion.
At each step, we randomly pick between image-text pre-training and Omni-Retrieval pre-training for updating the model parameters.
It takes in total 3,840 and 4,608 A100 hours to end-to-end pre-train our 6-layer CommerceMM and 12-layer CommerceMM with the vision encoder respectively.

\subsection{More Visualization}
We also visualize the text-to-image attention in Fig.~\ref{fig:attn_visualization}.
Comparing the the models pre-trained with 5 image-text tasks and all tasks (with Omni-Retrieval pre-training), we observe the cross-modal attention from all pre-training can better attend to the right regions referred by the key words, \eg, ``dress" and ``earrings".

\begin{figure}[h!]
    \centering
    \includegraphics[width=1.0\linewidth]{kdd22_commerceMM/figures/attn_visualization.png}
    \caption{Visualization of text-to-image attention from different pre-trained models.}
    \label{fig:attn_visualization}
\end{figure}
